# Supplementary material for: Dynamic Multi-level Privilege Control in Behavior-based Implicit Authentication Systems Leveraging Mobile Devices
Source: arXiv:1808.00638 source file (2021-04-15)
Supplement: Supplementary file 1 [file Appendix.pdf]

# 1 appendix

## 1.1 privilege movement

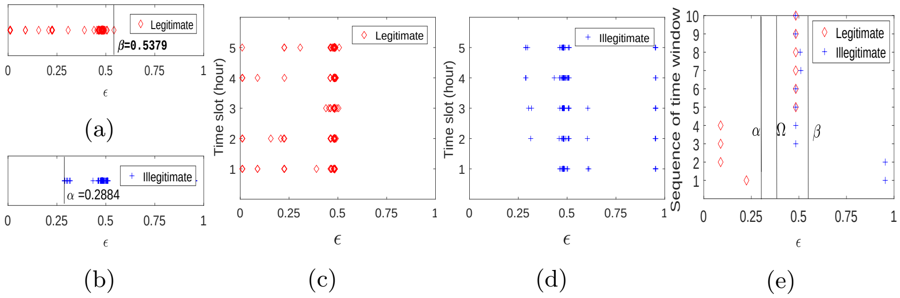


Figure 1: Behavior scores. (a) Behavior scores for legitimate user, (b) illegitimate user, (c) legitimate user in five time slots, (d) illegitimate user in five time slots, and (e) both users in the sequence of time window.

For the illegitimate user, as shown in Fig. 1, if system observes there are behavior scores fall in both illegitimate and slack domain at the same time and current privilege level is in the observation levels, the initial mapping may also be inaccurate, in which the current user may be illegitimate user and the system should lower the current privilege level. The chance of illegitimate usage increases when the number of behavior scores that fall into the illegitimate domain grows.

To further understand how *privilege movement* mechanism increases the accuracy, we randomly selected a time slot in Fig. 1 (c) and (d) and magnified it. We show the corresponding behavior scores in each time window in Fig. 1 (e) and corresponding false accept (FA) and reject (FR) results in Table 1, in which the time window indicates the time stamp for each authentication cycle. For example, in each time window, we tested the user once and recorded $\varepsilon$ for the test. We assume the very first user is legitimate. To simplify the discussion, we also assume the system contains only three privilege levels, top, observation and bottom privilege levels. After *initial mapping*, if the legitimate user has been mapped to observation level, as shown in Table 1 Case I, the system begins to monitor the behavioral change reflected by $\varepsilon$. The $\alpha$ and $\beta$ is predefined using historical data. As shown in the Fig. 1 (e), since the first behavior score of the legitimate user falls into the legitimate domain, the system moves the current privilege level upward toward the top privilege level with $-\mu_l = -\frac{l}{2}$. In the second time window, since the corresponding behavior score falls into the legitimate domain again, the system moves the current privilege level upward again, which reaches to the top privilege level in this time window. For rest time windows (3-10), although legitimate user has behavior score falls in slack domain, the system correctly identifies the current user as legitimate, in which the privilege level is still in the top privilege level since the behavior scores do

not fall in the illegitimate domain. After *initial mapping*, if the legitimate user has been mapped to the top privilege level, as shown in Table 1 Case II, the system will not change the current privilege level in the first two time windows. Same as the Case I, for the rest time windows (3-10), the privilege level also keeps in the top privilege level.
When illegitimate users have the device and current privilege level is at the top privilege level, in the first time window the system will move the current privilege level to observation level since the behavior score falls in the illegitimate domain as shown in Fig. 1 (e). In the next time window, the system moves the current privilege level to the last level and locks the device since it observes another behavior score falls in the illegitimate domain. In the rest of the time windows, the device will keep locked. It is also possible that the privilege level is at the observation level when illegitimate users have the device. The movement process is similar as the previous condition except that the device will be locked faster. For the traditional IA, the corresponding identification results are shown in Table. 1 at column TIA. The threshold $\Omega$ is predefined to best separate the two users. The traditional IA can not separate legitimate and illegitimate users in windows three to ten, in which it outputs at least two false accepts or false reject in time window 5, 6, 9 and 10 whatever we set the threshold. Similarly, in window 7 and 8 it produces at least two false accepts or false rejects. The *privilege movement* mechanism has the total false accepts and false rejects of 3, but traditional IA has 6. Generally, the behavior scores distribution may vary for different users, but the *privilege movement* mechanism can improve the identification accuracy in most of the time, especially when the first window contains the behavior score that falls in either legitimate or illegitimate domains, which is very common in practice. In practice, since it requires adversary several tried to fully imitate legitimate user's behavior, the current privilege level will be moved to the bottom before the adversary gains full control of the device. Similarly, the legitimate user is easy to be moved to the top privilege level if the training of the model is just finished, in which the legitimate user's behavior has little difference to the training data sampled recently and the corresponding behavior scores are easier to be mapped to the top level.

## 1.2 domain expansion for illegitimate user

Similar as the domain expansion for legitimate user, the expansion of illegitimate domain after user input a wrong password in the observation level is shown as,

$$S' = \frac{1}{2}(a' - \hat{a}')t^2 + v_0 t, \tag{1}$$

where $S'$ indicates the total displacement. $a'$ indicates the acceleration of the illegitimate domain expansion. $t$ indicates the number of time windows used in each authentication cycle. $v_0$ is initial velocity of the adjustment.

$$a' = \frac{1 - \varepsilon}{R_c * W_1} + W_2 + \delta', \tag{2}$$

Table 1: Test In Each Time Windows

| W* | Privilege Movement Mechanism | | | | TIA |
|---|---|---|---|---|---|
| | Legitimate Usage | | Illegitimate Usage | | FR+FA |
| | FR | | FA | | |
| | Case I | Case II | Case III | Case IV | |
| 1 | 1 | 0 | 1 | 0 | 0 |
| 2 | 1 | 0 | 0 | 0 | 0 |
| 3 | 0 | 0 | 0 | 0 | 0 |
| 4 | 0 | 0 | 0 | 0 | 0 |
| 5 | 0 | 0 | 0 | 0 | 1 |
| 6 | 0 | 0 | 0 | 0 | 1 |
| 7 | 0 | 0 | 0 | 0 | 1 |
| 8 | 0 | 0 | 0 | 0 | 1 |
| 9 | 0 | 0 | 0 | 0 | 1 |
| 10 | 0 | 0 | 0 | 0 | 1 |
| Sum | 2 | 0 | 1 | 0 | 6 |

*W indicates the sequence of time window. TIA indicates the traditional IA.

, where $1-\varepsilon$ indicates the distance between the behavior score and illegitimate domain; $\delta'$ represents the mixture of user behavior deviation and sensors' noise which correspond to two parameters of Kalman filter noted by process noise and observation noise respectively. $R_c$, $W_1$ and $W_2$ are same as described in section VI-B.

$$\hat{a}' = a'(\int_{\beta}^{1} p(\varepsilon_l)d\varepsilon_l + \theta'), \tag{3}$$

where $\beta$ denote the left bound of illegitimate domain; $\theta'$ is a constant; $\int_{\beta}^{1} p(\varepsilon_l)d\varepsilon_l$ indicates the chance that the illegitimate domain contains score derived from legitimate user in the training dataset, which can be estimated using *kernel density estimators*.
Similar as the discussion in section VI-B, we have,

$$S' = \frac{1}{2}a'(1 - \int_{\beta}^{1} p(\varepsilon_l)d\varepsilon_l - \theta') + v_0, \tag{4}$$

where the viscosity of the illegitimate domain is $(1 - \int_{\beta}^{1} p(\varepsilon_l)d\varepsilon_l - \theta')$, noted by $V'$.
Substituting Function 2 in Function 4, we have,

$$S = \frac{1}{2}(\frac{1-\varepsilon}{R_c * W_1} + W_2)V' + v_0 + \Delta' \tag{5}$$

where $\Delta' = \frac{V' * \delta'}{2}$ and it can be estimated using Kal-man filter.
